# Supplementary material for: None of the Above, Less of the Right: Parallel Patterns between Humans and LLMs on Multi-Choice Questions Answering
Source: arXiv:2503.01550 source file (2025-03-03)
Supplement: Supplementary file 1 [file sensitivity_study_of_mmlu_choices.tex]

\section{Lower bound of performance drop from MMLU}

In this section we study whether the drop from NA-as-answer was due to the
